# Supplementary material for: Machine Learning for Zombie Hunting: Predicting Distress from Firms' Accounts and Missing Values
Source: arXiv:2306.08165 source file (2023-06-13)
Supplement: Supplementary file 1 [file appendix.tex]

\section{Data Validation} \label{sec:appendixa}
\addcontentsline{toc}{section}{Appendix A}

To validate our dataset we can rely on the EUROSTAT data\footnote{EUROSTAT data used for our validation are available \href{http://ec.europa.eu/EUROSTAT/web/structural-business-statistics/data/database}{here}.}. EUROSTAT aggregates data coming from European national census bureaus and, with national differences, is the most reliable source of information on firm-level data for the countries in our sample. The dimensions that we used for the validation are the NACE sectoral classification and the number of people employed by size of the enterprise. While in a large number of cases the validation of the data is simply made by looking at the correlations between the working data and different data sources, here we develop a more ``accurate" mathematical validation for our data. 

Let $P_j^c$ be the proportion of observation within a cell $j$ defined by NACE sector or by the number of employees in the different firms' size classes\footnote{These two dimensions furnish alternative mean-squared-error measurement. For seek of brevity and to avoid burdening the terminology, we use just one index $j$ for the both cases, where $j=\{1,...,4\}$ in the case of number of employees by firm's size and $j=\{1,...,23\}$ in the case of NACE sector.} for a country $c$. We define the distance between the two data sources (ORBIS and EUROSTAT) for a country $c$, as the mean-squared-error between the proportions estimated in the ORBIS data $\hat{P}^{O,c}_{j}$ for country $c$ and the proportions in the EUROSTAT data ${P}^{E,c}_{j}$ for the same country:
\begin{equation}
MSE^c = {1 \over J}\sum_{j=1}^{J}\big(\hat{P}^{O,c}_{j} - {P}^{E,c}_{j}\big)^2
\end{equation}
where $\hat{P}^{O,c}_{j}$ is estimated, for instance in the case of the number of employees $\#e_k$ in a NACE sector $k$, as:
\begin{equation}
	\hat{P}^{O,c}_{k}= \frac{\#e_k}{\sum_{j=1}^{J}\#e_j} \:\:\: \text{with} \:\:\: k \in j.
\end{equation}
 Once we get all the mean-squared-errors per country both for NACE sectors and number of employees by firms size we test for the presence of outliers (namely, countries where the proportion of observation within different classes in EUROSTAT and ORBIS are significantly different). We do so in two ways: in one case we standardize the empirical distribution of the mean-squared-errors by country and then we test weather the single country mean-squared-error $MSE^c$ is significantly different from the empirical mean with a t-test; in another case we test for the presence of outliers by inter-quartile range\footnote{We consider a country's mean-squared-error to be an outlier when its value is above $Q_3 + 1.5	\cdot IQR$ of the empirical distribution.}. In both cases, Italian data do not fail the tests.

\section{Sensitivity of Predictions Analysis} \label{sec:appendixd}
\addcontentsline{toc}{section}{Appendix D}

In this paper, our identification strategy builds up on the ability of our favourite machine learning technique to provide accurate firms' level failure predictions. Hence, in this context the \textit{robustness} of machine learning predictions is central for our analysis. We argue that there is the need for specific techniques able to assess the \textit{sensitivity} of predictions as the usage of machine learning for prediction policy problems is strongly increasing in the last years \citep{kleinberg2015prediction, mullainathan2017machine}. 
The tasks of the \textit{sensitivity of predictions analysis} introduced here are mainly two:
\begin{enumerate}
			\item to assess how the omission of an unobserved confounder (orthogonal to the predictors) could affect the predictions of the model (\textit{stability});
			\item to assess if variations in the training population affect the predictions of the algorithm (\textit{generalizability}).
\end{enumerate}
 The stability check is directly inspired from the causal inference sensitivity analysis \citep{rosenbaum2005sensitivity, ichino2008temporary}. This analysis aims at assessing the impact of potential unobserved confounders on the model's predictions.
 The \textit{stability} of predictions is checked with respect to the estimated probabilities from our favorite BART model:
\begin{equation}
	f_{BART}(x) = \hat{p}_i(Y_i = 1 | X_i = x).
\end{equation}
 This \textit{stability} check is performed generating a new predictor (a \textit{confounder} $R_i$) and checking if (and how) the inclusion of it in the model changes the predicted probabilities of failure. This first check proceeds as follows:
\begin{enumerate}
			\item Create a \textit{confounder} $R_i$ with a higher correlation to $Y_i$ than the best predictor in the true model;
			\item Generate two models, one including just the observed predictors ($f^{true}_{BART}(x)$) and one including the observed predictors and the confounder $R_i$ ($f^{conf}_{BART}(x,r)$), on $b$ bootstrapped samples ($b=1,...,B$)\footnote{Clearly, we employ a bootstrap with replacement technique.}:
			\begin{eqnarray}
			(\text{i.})\:\:\:f^{true}_{BART}(x) &=& \hat{p}_{i,b}(Y_i = 1 | X_i = x) \\
			(\text{ii.})\:\:\:f^{conf}_{BART}(x,r) &=& \hat{p}_{i,b}(Y_i = 1 | X_i = x, R_i = r);
			\end{eqnarray}
			\item Check the \textit{distance} between:
			\begin{equation}
			 \hat{p}_{i,b}^{true} = \hat{p}_{i,b}(Y_i  = 1 | X_i = x) \:\: \text{and} \:\: \hat{p}_{i,b}^{conf} = \hat{p}_{i,b}(Y_i = 1 | X_i = x, R_i = r).
			\end{equation}
\end{enumerate}
The distance is checked on the sub-sample of units $i$ that are included in all the different bootstraped samples in 2 ways:
		\begin{enumerate}
			%\item overlap between the $\text{CI}_{95\%}$ of $\hat{p}_i^{true}$ and $\hat{p}_i^{conf}$ (in our case 98.37\%);
			
			\item $\text{T-test}_{99\%}$ if the null hypothesis of difference between the means of $\hat{p}_{i,b}^{true}$ and $\hat{p}_{i,b}^{conf}$ is rejected, where:
			
			\begin{equation}
			\hat{\bar{p}}_{i}^{true} = {1 \over B} \sum_{i=1}^{B} \hat{p}_{i,b}^{true} \:\:\: \text{and} \:\:\: \hat{\bar{p}}_{i}^{conf} = {1 \over B} \sum_{i=1}^{B} \hat{p}_{i,b}^{conf}
			\end{equation}

			\item standardized difference in means of $\hat{p}^{true}_{i,b}$ and $\hat{p}_{i,b}^{conf}$($\text{CI}_{95\%}$).
        \end{enumerate}

In the first case, the null hypotheses are rejected just 2.16\% of the times.       
Figure \ref{fig:sdm} depicts the results for the standardized differences in means for some randomly selected observations. The standardized differences in means are not significantly different from zero for all the $i$ observations in our sample.
			
The \textit{generalizability} check is performed by sub-sampling with replacement from the same population of observations and checking the stability of the unit level predictions $\hat{p}_{i,b}(Y_i  = 1 | X_i = x)$. Again, we use for the analysis the observations that are common to all the different sub-samples.
 This check proceeds as follows:
\begin{enumerate}
			\item Generate $B$ bootstrapped samples with replacement;
			\item Train $B$ BART models on every sample:
			\begin{equation}
			f_{BART}(x) = \hat{p}_{i,b}(Y_i = 1 | X_i = x);
			\end{equation}
			\item Check how many outliers are generated by looking at the following conditions:
		\end{enumerate}
\begin{eqnarray}
	\hat{p}_{i,b}(Y_i = 1 | X_i = x) &\geq& \bar{\hat{p}}_i(Y_i = 1 | X_i = x) + 2 \cdot sd(\hat{p}_{i}(Y_i = 1 | X_i = x)) \\
	&\text{or}& \nonumber \\
	\hat{p}_{i,b}(Y_i = 1 | X_i = x) &\leq& \bar{\hat{p}}_i(Y_i = 1 | X_i = x) - 2 \cdot sd(\hat{p}_{i}(Y_i = 1 | X_i = x)).
\end{eqnarray}
Following this procedure we found 5.27\% of outliers in the predictions. Figure \ref{fig:bp} depicts the box plots for the failure probabilities of randomly selected observations. As we can see, the distributions are very shrieked.
