# Supplementary material for: Machine Learning for Zombie Hunting: Predicting Distress from Firms' Accounts and Missing Values
Source: arXiv:2306.08165 source file (2023-06-13)
Supplement: Supplementary file 2 [file online_appendix.tex]

\section*{Appendix C: Variables Selection with LASSO}

In previous analyses, we explicitly claimed that we needed as much in-sample information as possible to reduce out-of-sample errors in predictions. On the other hand, there could be problems of overfitting when data dimensionality increases\footnote{The so-called \textit{curse of dimensionality} is an obstacle in many cases, when one works with finite data samples and many variables. The seminal reference is to the work by \cite{bellman_adaptive}, who introduced the notion of dimensionality reduction.}. In this Section, we show what happens when we sift through firm-level data and try to extract a set of predictors with the highest ability to spot financial distress.
The natural candidate tool to shrink the dimensionality of a matrix of predictors is the LOGIT-LASSO \citep{ahrens2019lassopack}, whose functional form in a panel setting is the following:
\begin{eqnarray}\label{eq:LOGITLASSO}
\argmin_{{\beta} \in \mathbb{R}^{p}} \:\: \frac{1}{2N} \sum_{i=1}^N \left(y_{i,t}(x_{i,t-1}^T\beta) - log(1 + e^{(x_{i,t-1}^T\beta)})\right)^2 \:\:\:
{\rm subject\,\,to\,\,} \|{\beta}\|_1 \leq k.
\end{eqnarray}
where $y_{i,t}$ is a binary variable equal to one if a firm $i$ failed at time $t$ and zero otherwise. Any $x_{i,t-1}$ is a lagged predictor chosen in $\mathbb{R}^{p}$ at time $t-1$, whereas $\|{\beta}\|_1=\sum_{j=1}^p |\beta_j|$ and $k > 0$. The constraint $\|{\beta}\|_1 \leq k$ limits the complexity of the model to avoid overfitting, and $k$ is chosen, following \citet{ahrens2019lassopack}, as the value that maximises the Extended Bayesian Information Criteria \citep{chen2008extended}. To account for the potential presence of heteroskedastic, non-Gaussian and cluster-dependent errors, we adopt the rigorous penalization introduced by \cite{belloni2016inference}. Top ten highest-ranked predictors are presented in Table \ref{tab:predictors_of_failure}.

Even though number of predictors varies in time, up to a maximum of twenty-one features in 2015, we find a core set of predictors that are frequently selected. The stable set includes indicators of financial distress (\textit{Liquidity Returns, Interest Coverage Ratio, Interest Benchmark, Financial Constraint}), as well as indicators related to the core economic activities of the firms (\textit{Negative Value Added, Total Factor Productivity, Size-Age}). Apparently, firms that are controlled by parent companies (\textit{Corporate Control}) are less likely to fail in every period, i.e., the predictor enters in the algorithm with a negative coefficient. The same happens for the \textit{Dummy Trademarks} and the \textit{Dummy Patents}, as it makes sense that intangible assets reduces the probability to exit from the market\footnote{See Table \ref{tab:table2} for a full description of predictors and their construction.}.
\pagebreak

\begin{landscape}
\vspace*{27mm}

\begin{table}[H]
\centering
\doublespacing
\caption{Top 10 predictors for firms' failures - Results from a rigorous LOGIT-LASSO}
\label{tab:predictors_of_failure}
	\resizebox{1.3\textwidth}{!}{%
		\begin{tabular}{cccccccccc}
		\toprule
			Rank & 2017                         & 2016                    & 2015                             & 2014                             & 2013                             & 2012                             & 2011            & 2010  & 2009               \\
			\midrule
		    1                           & Liquidity Returns           & Negative Value Added & Negative Value Added &  Negative Value Added & Liquidity Returns  & Negative Value Added    &   Negative Value Added & Negative Value Added  & Negative Value Added  \\
			2                           & Negative Value Added  & Liquidity Returns          & Corporate Control    &  Liquidity Returns         & Negative Value Added & Profitability  &  Liquidity Returns  & Liquidity Returns & Liquidity Returns \\
			3                           & Corporate Control      & Corporate Control     & Financial Constraint        & Solvency Ratio  & Solvency Ratio  & Financial Constraint &  Financial Constraint & Profitability & Financial Constraint       \\
			4                           & Interest Coverage Ratio          & Financial Constraint         & Interest Coverage Ratio        & Profitability &  Profitability & Corporate Control & Corporate Control    & Financial Constraint          & Profitability\\
			5                           & Financial Constraint         & Interest Coverage Ratio         & Profitability & Financial Constraint       & Corporate Control    & Solvency Ratio & Solvency Ratio     & Corporate Control      & Corporate Control \\
			6                           & Solvency Ratio     & Size-Age    &  Solvency Ratio   & Corporate Control   & Financial Constraint        & Interest Coverage Ratio & Size-age     & Solvency Ratio     & Solvency Ratio \\
			7                           & Size-age     & Solvency Ratio    & Size-age     & Size-age  & Size-Age   & Liquidity Returns & Interest Coverage Ratio          & Region (NUTS 2)         & Interest Coverage Ratio \\
			8                           & Profitability & Profitability &  Interest Benchmark        & Interest Coverage Ratio       & Interest Coverage Ratio       & Size-age & Financial Misallocation & Dummy Trademarks    & Dummy Trademarks\\
			9                           & Interest Benchmark          & Interest Benchmark          &  Liquidity Ratio  & TFP       & TFP        & Dummy Patents & Dummy Trademarks    & Interest Coverage Ratio          & Size-age\\
			10                          & Liquidity Ratio    & Liquidity Ratio    & Capital Intensity          & Liquidity Ratio & Dummy Patents & Dummy Trademarks & Dummy Patents   & Dummy Patents   & Capital Intensity \\
			\bottomrule
		\end{tabular}
		}
		\begin{tablenotes}
\footnotesize
\singlespacing
\item Note: The rankings are obtained after the implementation of a rigorous LOGIT-LASSO \citep{robustlasso, belloni2016post} every year on the entire battery of predictors described in Figure \ref{tab:table2}. Only the first ten selections are reported. The procedure selects a different number of predictors every year, up to a maximum of 21.
\end{tablenotes}
\end{table}
\end{landscape}

Some of the top predictors we show have been used to measure either financial distress or \textit{zombie lending}. However, the ranking changes over time, and we do not detect any meaningful pattern in these changes. In this context, we cannot rely on a single indicator (or a set thereof) to derive predictions of failures. If we did, we would have a higher rate of \textit{false positives} (when our forecasts indicate that a firm is at risk of failure, but it is not) and a higher rate of \textit{false negatives} (when the predictions wrongly suggest that a firm in trouble deserves credit).

In fact, at this stage, we cannot exclude that a different ranking over time is due to better use of the newly acquired in-sample information after new failures have been observed. Also, it might be the case that a change in rankings reflects some shift in the business environment in which companies operate. We presume that applications to different aggregates (countries, regions, industries) may return different rankings.
In the spirit of a pure prediction problem, we conclude that it is better to keep the entire battery of predictors, as far as a dimensionality problem on the predictors does not arise, when we can train predictions on a large enough number of firm-level observed outcomes.

\section{Robustness checks: indicators selection} \label{sec:indicators_selection}
\addcontentsline{toc}{section}{Appendix E}

A possible drawback is that this method could tend to select just the best predictors of firms failures since our indicator is based on predicted probabilities of failures. Thus, we developed a ``two-stages" method to possibly overcome this sort of problem. In the first stage, we use a LOGIT model to predict which firms should and should not fail according to the model. In the second stage we select, again through a LOGIT-LASSO regression, the best predictors for false positives. Namely, which are the variables that predict the status of a firm that should fail but is yet surviving. We argue that both these definitions are strongly connected with the \textit{survival} definition of \textit{zombie} firms. 

Here, we run both the Logistic regression (first stage) and the LASSO (second stage) using the status observed at time $t$ (either the time of failure, for the failed firms, or 2017 for the not-failed firms) and the predictors at time $t-1$ (either the year before failure, for the failed firms, or 2016 for the not-failed firms).
Thought this analysis we were able to spot the variables that best predict the survival of a firm that has a ``high-similarity" with other failed firms. The variables that have the best predictive power are \textit{control}, \textit{solvency}, \textit{BID}, \textit{negative added value}, \textit{profitability}, \textit{liquidity return}.

These results on one side provide a further validation of some of indicators that were found to be good predictors also in the first method (\textit{control}, \textit{solvency}, \textit{negative added value}, \textit{profitability}, \textit{liquidity return}) and on the other side highlights a strong role of the \textit{BID} indicator by \cite{caballero2008zombie} as a drivers of the \textit{zombie} phenomenon in Italy. Further details on this methodology are provided in the online Appendix.
