# Supplementary material for: Machine Learning for Zombie Hunting: Predicting Distress from Firms' Accounts and Missing Values
Source: arXiv:2306.08165 source file (2023-06-13)
Supplement: Supplementary file 3 [file additional_and_old_analysis.tex]

\documentclass[11pt]{article}\usepackage{amssymb,amsmath,amsfonts,eurosym,geometry,ulem,graphicx,caption,color,setspace,sectsty,comment,footmisc,caption,natbib,pdflscape, array, graphicx, subcaption, float, booktabs, appendix, tabularx, mathtools, threeparttable, lscape, enumerate, bbm, tikz-qtree, rotating, color}
\usepackage{hyperref}
\hypersetup{
colorlinks=true,
citecolor=blue,
linkcolor=blue,
filecolor=blue,      
urlcolor=blue,
}



\normalem

\onehalfspacing
\newtheorem{theorem}{Theorem}
\newtheorem{corollary}[theorem]{Corollary}
\newtheorem{proposition}{Proposition}
\newenvironment{proof}[1][Proof]{\noindent\textbf{#1.} }{\ \rule{0.5em}{0.5em}}

\newtheorem{hyp}{Hypothesis}
\newtheorem{subhyp}{Hypothesis}[hyp]
\renewcommand{\thesubhyp}{\thehyp\alph{subhyp}}

\newcommand{\red}[1]{{\color{red} #1}}
\newcommand{\blue}[1]{{\color{blue} #1}}

\DeclareMathOperator*{\argmax}{arg\,max}
\DeclareMathOperator*{\argmin}{arg\,min}
\newcommand{\bX}{\mathbf{X}}

\newcolumntype{L}[1]{>{\raggedright\let\newline\\arraybackslash\hspace{0pt}}m{#1}}
\newcolumntype{C}[1]{>{\centering\let\newline\\arraybackslash\hspace{0pt}}m{#1}}
\newcolumntype{R}[1]{>{\raggedleft\let\newline\\arraybackslash\hspace{0pt}}m{#1}}

\geometry{left=1.0in,right=1.0in,top=1.0in,bottom=1.0in}

\begin{document}

\newpage
\section*{Appendix E: Missing Imputation Analysis}\label{appendix:threshold}


\subsection*{E.3 K-Nearest Neighbors (KNN) median-based imputation}
We perform imputation using the median of the $K = 5$ nearest neighbours of each case observation with missing values. We use the median for continuous variables and the mode for categorical ones. 

\begin{table}[H]
\centering
    \begin{tabular}{lcccccc}
\hline 
 Method &  ROC  &  PR  &  F1-Score  &  BACC  &  $R^2$  &  Time \\ \hline \hline 
\textit{Logit CC} &  0.8798 &  0.2047 &  0.0788 &  0.7477  &  0.1065  &  10.71 \\
\textit{Logit} &  0.8537  &  0.3101 &  0.1349  &  0.7158  &  0.1815 &  34.30  \\ 
\textit{Ctree}  &   0.9589  &  0.6758  &  0.1353  &  0.7719  &  0.4734  &  2115.82 \\ 
\textit{RF}   &  0.9856  &  0.8514  &  0.1914  &  0.8509  &  0.6496  &  810.73 \\ 
\textit{XGBoost} &   0.9650  &  0.6594  &  0.1737  &  0.8300  &  0.4492  &  2.49  \\ 
\textit{BART}  &  0.9733  &  0.7225  &  0.1267  &  0.7573  &  0.5152  &  5463.72  \\ 
\textit{SL} &   0.9894  &  0.8771  &  0.1271  &  0.7588  &  0.6988  &  13749.46  \\ 
\textit{BART-MIA} & 0.9768 &  0.7468  &  0.1277  &  0.7599  &  0.5308  &  4664.73 \\ \hline  
\end{tabular}
\caption{Model performances with KNN imputed data. All the algorithms are trained with five-fold cross-validation. The training and test set respectively involve 238,148 and 59,537 observations in each iteration. Only the \textit{BART-MIA} and the \textit{Logit CC} differ in the reported train and test sets since their cross-validation is respectively built  on the original dataset with missing values and on the complete-case version resulting from listwise deletion. All the metrics correspond to the five fold average. Time represents the average seconds required to train the model in each fold. Train and test represents the number of observations involved in each step of the cross-validation process.}
\end{table}

\begin{table}[H]
    \centering
    \begin{tabular}{ccccc}
    \hline
\textit{Logit} & \textit{CTree} & \textit{RF} & \textit{XGBoost} & \textit{BART} \\ \hline
 0  &  0  &  0.2653  &  0.7347  &  0  \\ \hline
\end{tabular}
\caption{The SL distribution of the optimal coefficients for uniform median imputation.}
\end{table}

\newpage
\subsection*{E.4 Uniform median sampling imputation}
We impute the missing values of a variable $q$ by sampling from a continuous uniform distribution with bounded support on $[q_{.5}-s_n, \ q_{.5}+s_n]$, where $q_{.5}$ and $s_n$ are respectively the median and the sample standard deviation of the observed distribution of $q$.
\begin{table}[H]
\centering
    \begin{tabular}{lcccccc}
\hline 
 Method &  ROC  &  PR  &  F1-Score  &  BACC  &  $R^2$  &  Time \\ \hline \hline 
\textit{Logit CC} &  0.8798 &  0.2047  &  0.0788 &  0.7477  &  0.1065  &  10.71 \\
\textit{Logit} & 0.9061 & 0.2905 & 0.1261 & 0.7548 & 0.1573 & 27.63  \\ 
\textit{Ctree}  &  0.9187  &  0.3501  &  0.1618  &  0.8132  &  0.1985  &  1763.59  \\ 
\textit{RF}   &   0.9698  &  0.6956  &  0.1396  &  0.7823  &  0.4609  &  753.82  \\ 
\textit{XGBoost} &  0.9617  &  0.6556  &  0.1671  &  0.8221  &  0.4390  &  2.77  \\ 
\textit{BART}  &   0.9678   &   0.6325   &   0.1268  &   0.7577   &   0.4236   &   4533.20 \\ 
\textit{SL} &    0.9767   &   0.7431   &   0.1269   &   0.7581   &   0.5280   &   15550.71   \\ 
\textit{BART-MIA} & 0.9768 &  0.7468  &  0.1277  & 0.7599  & 0.5308  &  4664.73 \\ \hline  
\end{tabular}
\caption{Model performances with uniform median imputed data. All the algorithms are trained with five-fold cross-validation. The training and test set respectively involve 238,148 and 59,537 observations in each iteration. Only the \textit{BART-MIA} and the \textit{Logit CC} differ in the reported train and test sets since their cross-validation is respectively built  on the original dataset with missing values and on the complete-case version resulting from listwise deletion. All the metrics correspond to the five fold average. Time represents the average seconds required to train the model in each fold. Train and test represents the number of observations involved in each step of the cross-validation process.}
\end{table}

\begin{table}[H]
    \centering
    \begin{tabular}{ccccc}
    \hline
\textit{Logit} & \textit{CTree} & \textit{RF} & \textit{XGBoost} & \textit{BART} \\ \hline
  0  &  0.0720  &  0.2334  &  0.6936  &  0.0011  \\ \hline 
\end{tabular}
\caption{The SL distribution of the optimal coefficients for uniform median sampling imputation.}
\end{table}


\subsection*{\textcolor{red}{XGBoost performance for moving cutoffs}}
I report performance metrics related to XGBoost predictions of failure according to different classification thresholds. I deal with the problem with five fold cross-validation. The model is trained five times for each cutoff, and performance metrics are computed on the corresponding test set. Therefore, each row of Table 1 provides the average of the metrics over the five fold (for a given cutoff). Note that positives corresponds to failed firms and negative those not. 
\begin{table}[H]
\centering
   \begin{tabular}{|c|c|c|c|c|c|c|c|}
    \hline 
        Cutoff  &  PPV  &  TPR  &  BACC  & \textbf{TN} & \textbf{FP} & \textbf{FN} & \textbf{TP} \\ \hline \hline
          0.60   &   0.0971   &   0.9897   &   0.8328   &   38869   &   18648   &    21   &   1999   \\ \hline
          0.61   &   0.0971   &   0.9897   &   0.8328   &   38869   &   18648   &    21   &   1999   \\ \hline
          0.62   &   0.0971   &   0.9897   &   0.8328   &   38869   &   18648   &    21   &   1999   \\ \hline
          0.63   &   0.0971   &   0.9897   &   0.8328   &   38869   &   18648   &    21   &   1999   \\ \hline
          0.64   &   0.1009   &   0.9890   &   0.8398   &   39716   &   17802   &    22   &   1997   \\ \hline
          0.65   &   0.1009   &   0.9890   &   0.8398   &   39716   &   17802   &    22   &   1997   \\ \hline
          0.66   &   0.1009   &   0.9890   &   0.8398   &   39716   &   17802   &    22   &   1997   \\ \hline
          0.67   &   0.1359   &   0.9890   &   0.8842   &   44822   &   12695   &    22   &   1997   \\ \hline
          0.68   &   0.1359   &   0.9890   &   0.8842   &   44822   &   12695   &    22   &   1997   \\ \hline
          0.69   &   0.1359   &   0.9890   &   0.8842   &   44822   &   12695   &    22   &   1997   \\ \hline
          0.70   &   0.1359   &   0.9890   &   0.8842   &   44822   &   12695   &    22   &   1997   \\ \hline
          0.71   &   0.1359   &   0.9890   &   0.8842   &   44822   &   12695   &    22   &   1997   \\ \hline
          0.72   &   0.1359   &   0.9890   &   0.8842   &   44822   &   12695   &    22   &   1997   \\ \hline
          0.73   &   0.1359   &   0.9890   &   0.8842   &   44822   &   12695   &    22   &   1997   \\ \hline
          0.74   &   0.1359   &   0.9890   &   0.8842   &   44822   &   12695   &    22   &   1997   \\ \hline
          0.75   &   0.1359   &   0.9890   &   0.8842   &   44822   &   12695   &    22   &   1997   \\ \hline
          0.76   &   0.1492   &   0.9824   &   0.8926   &   46177   &   11341   &    36   &   1984   \\ \hline
          0.77   &   0.1492   &   0.9824   &   0.8926   &   46177   &   11341   &    36   &   1984   \\ \hline
          0.78   &   0.2091   &   0.9393   &   0.9031   &   49866   &    7651   &   122   &   1897   \\ \hline
          0.79   &   0.2091   &   0.9393   &   0.9031   &   49866   &    7651   &   122   &   1897   \\ \hline
          0.80   &   0.2121   &   0.9393   &   0.9049   &   50072   &    7445   &   122   &   1897   \\ \hline
          0.81   &   0.2121   &   0.9393   &   0.9049   &   50072   &    7445   &   122   &   1897   \\ \hline
          0.82   &   0.2655   &   0.9087   &   0.9102   &   52439   &    5078   &   184   &   1835   \\ \hline
          0.83   &   0.2655   &   0.9087   &   0.9102   &   52439   &    5078   &   184   &   1835   \\ \hline
          0.84   &   0.2655   &   0.9087   &   0.9102   &   52439   &    5078   &   184   &   1835   \\ \hline
          0.85   &   0.2655   &   0.9087   &   0.9102   &   52439   &    5078   &   184   &   1835   \\ \hline
          0.86   &   0.2655   &   0.9087   &   0.9102   &   52439   &    5078   &   184   &   1835   \\ \hline
          0.87   &   0.2655   &   0.9087   &   0.9102   &   52439   &    5078   &   184   &   1835   \\ \hline
          0.88   &   0.2655   &   0.9087   &   0.9102   &   52439   &    5078   &   184   &   1835   \\ \hline
          0.89   &   0.2863   &   0.9010   &   0.9110   &   52981   &    4536   &   200   &   1819   \\ \hline
          0.90   &   0.3130   &   0.8770   &   0.9046   &   53626   &    3892   &   249   &   1771   \\ \hline
          0.91   &   0.3331   &   0.8652   &   0.9022   &   54017   &    3501   &   272   &   1747   \\ \hline
          0.92   &   0.3628   &   0.8457   &   0.8968   &   54517   &    3001   &   312   &   1708   \\ \hline
          0.93   &   0.3973   &   0.8175   &   0.8870   &   55013   &    2504   &   369   &   1651   \\ \hline
          0.94   &   0.4956   &   0.7192   &   0.8460   &   55951   &    1567   &   567   &   1453   \\ \hline
          0.95   &   0.5896   &   0.6343   &   0.8094   &   56625   &     892   &   739   &   1281   \\ \hline
    \end{tabular}
\caption{Precision/Positive Predictive Value (PPV), Recall/True Positive Rate (TPR), F1-Score and Balanced Accuracy (BACC) performances of XGBoost and the corresponding confusion matrices reporting the number of True Negatives (TN), False Positives (FP), False Negatives (FN), True Positives (TP).}
\end{table}






\newpage
\section*{\textcolor{red}{Encoding missingness}}
We perform complete-case analysis and different encoding strategies to deal with missingness. As we agreed, \textbf{we exclude firms in liquidation} from the analysis according to the comment 2 of Referee II (page 16). \\ \\
Note: the Super Learner (\textit{SL}) is the ensemble model of \textit{Logit}, Conditional Inference Tree (\textit{CTree}), Random Forest (\textit{RF}), a non-tuned Extreme Gradient Boosting (\textit{XGBoost}) and Bayesian Additive Regression Tree (\textit{BART}) with no Missingness Incorporated in Attributes (\textit{MIA}). \textit{FT-XGBoost} denotes the \textit{XGBoost} model with fine-tuned hyperparameters. 
\subsection*{\textcolor{blue}{0) Complete-case (CC) analysis}}
We initially perform a CC analysis, a standard routine when the model is not designed to deal with missing values. All the observations containing at least one missing value in the predictors are dropped. The initial number of sample failures (\textbf{net of liquidations}) is 10,098. The CC analysis leads to the loss of 8.163 observations, which corresponds to the 80.84\% of the initial sample failures. For the sake of comparison, we train a correspondent \textit{XGBoost} and \textit{BART-MIA} model with 5-fold cross-validation on a random sample of the same dimension from the original data with missing values. Therefore, observations now involve missing values in the predictors.  
\begin{table}[H]
\centering
    \begin{tabular}{|l|c|c|c|c|c|r|}
\hline 
\multicolumn{1}{|c|}{\textbf{No missing}}  &  ROC  &  PR  &  F1-Score  &  BACC  &  $R^2$  &  Time \\ \hline
\textit{Logit} &  0.8798  &  0.2047  &  0.0788  &  0.7477  &  0.1065  &  10.71 \\ \hline
\textit{Ctree}  &  0.8744  &  0.1930  &  0.0851  &  0.7663  &  0.1070  &  379.73  \\ \hline
\textit{RF}   &      0.8967   &   0.2991   &   0.0898  &   0.7716  &   0.1630   &   192.18   \\ \hline
\textit{XGBoost} &  0.9027  &  0.2774  &  0.0788  &  0.7477  &  0.1475 &  33.51    \\ \hline
\textit{BART}   &  0.9079  &  0.2896  &  0.0789  &  0.7488  &  0.1636  &  1128.94  \\ \hline
\textit{SL} &  0.9152 &  0.3254  &  0.0789  &  0.7485  &  0.1866  &  4129.14 \\ \hline
\multicolumn{7}{c}{} \\ \hline
\multicolumn{1}{|c|}{\textbf{Missing}} &  ROC  &  PR  &  F1-Score  &  BACC  &  $R^2$  &  Time \\ \hline
\textit{XGBoost} &     0.9753   &   0.7463   &   0.1282   &   0.7583   &   0.5292   &   36.51    \\ \hline
\textit{BART-MIA} & 0.9750 & 0.7364 & 0.1262 & 0.7596 & 0.5216 & 1292.80 \\ \hline
\multicolumn{7}{c}{} \\ \hline
\multicolumn{1}{|c|}{Train} & \multicolumn{6}{c|}{74,340} \\
\hline
\multicolumn{1}{|c|}{Test} & \multicolumn{6}{c|}{18,585} \\ \hline
\end{tabular}
\caption{Model performances with CC data. All the algorithms are trained with five-fold cross validation. All the metrics correspond to the five fold average. Time represents the average seconds required to train the model in each fold. Train and test represents the number of observations involved in each step of the cross-validation process.}
\end{table}

\begin{table}[H]
    \centering
    \begin{tabular}{|c|c|c|c|c|}
    \hline
 \textit{Logit} & \textit{CTree} & \textit{RF} & \textit{XGBoost} & \textit{BART} \\ \hline
 0.0354   &   0.0138   &   0.4809  &   0.3289   &   0.1411  \\ \hline
\end{tabular}
\caption{The SL distribution of the optimal coefficients for CC imputation.}
\end{table}

\subsection*{\textcolor{blue}{0.1) CC analysis with liquidations}} 
\begin{table}[H]
\caption{Model performances: CC analysis}
\label{tab:cc_analysis}
\centering
    \begin{tabular}{lcccccc}
\hline 
\multicolumn{1}{c}{Method}  &  AUC  &  PR  &  F1-Score  &  BACC  &  $R^2$  &  Time \\ \hline \hline  
\textit{Logit} &     0.8966   &   0.4542   &   0.1833   &   0.7504   &   0.2658   & 9.13 \\ 
\textit{Ctree}  &   0.8957  &   0.4444   &   0.1987   &   0.7668   &   0.2640  &   572.46    \\ 
\textit{Random Forest}  &   0.9117   &   0.5233   &   0.1907   &   0.7595   &   0.3135  &   261.62    \\ 
\textit{XGBoost} &    0.9140   &   0.5170   &   0.1833   &   0.7504   &   0.3126 &   43.66    \\ 
\textit{BART}   &    0.9185  &   0.5221   &   0.1843   &   0.7533   &   0.3179   &   1249.05    \\ 
\textit{Super Learner} &   0.9231   &   0.5464   &   0.1844   &   0.7535   &   0.3373   &   4147.87   \\ \hline 
\end{tabular}
\end{table}

\begin{table}[H]
\caption{Model performances: Missing-aware analysis}
\label{tab:missing_aware_analysis}
\centering
    \begin{tabular}{lcccccc}
\hline 
\multicolumn{1}{p{\widthof{Random Forest}}}{Method} &  AUC  &  PR  &  F1-Score  &  BACC  &  $R^2$  &  Time \\ \hline \hline
\textit{XGBoost} &  0.9685     &     0.7591  &  0.2070     &     0.7646     &   0.5243  &  24.70    \\
\textit{BART-MIA} &   0.9681   &    0.7516  &  0.2092 &    0.7676   &    0.5178    &    1126.88    \\ \hline
%\multicolumn{1}{|c|}{Train} & \multicolumn{6}{c|}{74,340} \\
%\hline
%\multicolumn{1}{|c|}{Test} & \multicolumn{6}{c|}{18,585} \\ \hline
\end{tabular}
\end{table}
\begin{tablenotes}
\footnotesize
\item All the algorithms are trained with five-fold cross-validation. The training and test set respectively involve 95,970 and 19,194 observations in each iteration. All the metrics correspond to the five-fold average. Time represents the average seconds required to train the model in each fold. Train and test represent the number of observations involved in each step of the cross-validation process. 
\end{tablenotes}



\newpage
\subsection*{\textcolor{blue}{1) Out-of-range values imputation}}
We impute all the missing values in the dataset with an out-of-range value, i.e. $10^{20}$. 
\begin{table}[H]
\centering
    \begin{tabular}{|l|c|c|c|c|c|r|}
\hline 
  &  ROC  &  PR  &  F1-Score  &  BACC  &  $R^2$  &  Time \\ \hline
\textcolor{blue}{\textit{Logit CC}} &  \textcolor{blue}{0.8798}  &  \textcolor{blue}{0.2047 } &  \textcolor{blue}{0.0788 } &  \textcolor{blue}{0.7477}  &  \textcolor{blue}{0.1065}  &  \textcolor{blue}{10.71} \\ \hline
\textit{Logit}  &  0.9657  &  0.6689  &  0.1270 &  0.7588  &  0.4558  &  56.49 \\ \hline
\textit{Ctree}  &  0.9712  &  0.6999  &  0.1323  &  0.7686  &  0.4840  &  1628.08 \\ \hline 
\textit{RF}   &   0.9343  &   0.7000  &   0.2011   &   0.8371  &   0.4999   &   608.33  \\ \hline
\textit{XGBoost} &  0.9691   &    0.7172    &    0.1767    &    0.8327    &    0.5030   &    2.65  \\ \hline 
\textcolor{red}{\textit{FT-XGBoost}} &   \textcolor{red}{0.9792}  &   \textcolor{red}{0.7619} &   \textcolor{red}{0.1270 } &   \textcolor{red}{0.7585}  &   \textcolor{red}{0.5461}  &   \textcolor{red}{34.27}  \\ \hline
\textit{BART}   &   0.9770  &  0.7482  &  0.1296  & 0.7635   &  0.5327  & 2736.74   \\ \hline
\textit{SL}  &  0.9788  &  0.7574  &  0.1289  &  0.7626  &  0.5454  &  11765.18   \\ \hline 
\textcolor{red}{\textit{BART-MIA}} & \textcolor{red}{0.9768} &  \textcolor{red}{0.7468}  &  \textcolor{red}{0.1277}  &  \textcolor{red}{0.7599}  &  \textcolor{red}{0.5308}  &  \textcolor{red}{4664.73}  \\ \hline  
\multicolumn{7}{c}{} \\ \hline
\multicolumn{1}{|c|}{Train} & \multicolumn{6}{c|}{238,148 obs.} \\
\hline
\multicolumn{1}{|c|}{Test} & \multicolumn{6}{c|}{59,537 obs.} \\ \hline
\end{tabular}
\caption{Model performances with out-of-range values imputed data. All the algorithms are trained with five-fold cross-validation. Only the \textit{BART-MIA} and the \textit{Logit CC} differ in the reported train and test sets since their cross-validation is respectively built  on the original dataset with missing values and on the complete-case version resulting from listwise deletion. All the metrics correspond to the five fold average. Time represents the average seconds required to train the model in each fold. Train and test represents the number of observations involved in each step of the cross-validation process.}
\end{table}

\begin{table}[H]
    \centering
    \begin{tabular}{|c|c|c|c|c|}
    \hline
 \textit{Logit} & \textit{CTree} & \textit{RF} & \textit{XGBoost} & \textit{BART} \\ \hline
  0.3214   &   0.0991   &   0.3344   &   0.2273   &   0.0969 \\ \hline 
\end{tabular}
\caption{The SL distribution of the optimal coefficients for out-of-range values imputation.}
\end{table}

\begin{table}[H]
    \centering
    \begin{tabular}{|c|c|c|c|c|}
    \hline
\textit{booster} & \textit{max\textunderscore depth} & \textit{min\textunderscore child\textunderscore weight} & \textit{subsample} & \textit{colsample\textunderscore bytree} \\ \hline
gbtree & 7 & 4.5363 & 0.9877 & 0.8210 \\ \hline
\end{tabular}
\caption{The XGBoost values for the optimal parameters when fine-tuned.}
\end{table}
Regarding \textit{XGBoost}, we first train a ``naive  version of it, with no hyperparameters tuning and setting the maximum number of boosting iterations equal to five to speed up the process. Secondly, we perform hyperparameters tuning as follows: we determine the best number of iteration with 5-fold CV using the in-built \textit{xgb.cv} function; having set the optimal number of iterations, we proceed with 5-fold CV in random search of the following hyperparameters:
\begin{itemize}
    \item \textit{booster}: it governs which model to use (\textit{gbtree}, \textit{gblinear} or \textit{dart}). 
    \item \textit{min\textunderscore child\textunderscore weight}: a stopping rule for tree splitting. If the leaf node has a minimum sum of instance weight (calculated by second order partial derivative) lower than \textit{min\textunderscore child\textunderscore weight}, the tree splitting stops.
    \item \textit{subsample}: it controls the number of observations supplied to a tree. Setting it to 0.5 means that XGBoost would randomly sample half of the training data prior to growing trees. This will prevent overfitting. Subsampling occurs once for every tree constructed
    \item \textit{colsample\textunderscore bytree}: it specifies the fraction of columns to be subsampled. It controls for the number of features supplied to a tree, like in Random Forest.
\end{itemize}
In this last stage of CV, we also exploit stratification, which ensures that the distribution of failures is mantained in the resample datasets. 







\newpage
\subsection*{\textcolor{blue}{2) Median imputation}}
We impute the missing values of a variable $q$ with its median $q_{.5}$.
\begin{table}[H]
\centering
    \begin{tabular}{|l|c|c|c|c|c|r|}
\hline 
  &  ROC  &  PR  &  F1-Score  &  BACC  &  $R^2$  &  Time \\ \hline
\textcolor{blue}{\textit{Logit CC}} &  \textcolor{blue}{0.8798}  &  \textcolor{blue}{0.2047 } &  \textcolor{blue}{0.0788 } &  \textcolor{blue}{0.7477}  &  \textcolor{blue}{0.1065}  &  \textcolor{blue}{10.71} \\ \hline
\textit{Logit} &  0.8825  &  0.2690 &  0.1465  &  0.7540  &  0.1495  &  50.77  \\ \hline
\textit{Ctree}  &  0.9270  &  0.4017  &  0.1492  &  0.7962  &  0.2364  &  1975.38  \\ \hline 
\textit{RF}   &  0.7767  &  0.4337  &  0.1487  &  0.7060  &  0.2667  &  855.37   \\ \hline
\textit{XGBoost} &  0.9480  &  0.4779  &  0.1830  &  0.8394  &  0.2940  &  2.05   \\ \hline 
\textit{BART}   &  0.9485  &  0.4936  &  0.1328  &  0.7688  &  0.3014  &  4345.19    \\ \hline
\textit{SL} &  0.9595  &  0.5393  &  0.1269  &  0.7576  &  0.3389  &  13927.68    \\ \hline 
\textcolor{red}{\textit{BART-MIA}} & \textcolor{red}{0.9768} &  \textcolor{red}{0.7468}  &  \textcolor{red}{0.1277}  &  \textcolor{red}{0.7599}  &  \textcolor{red}{0.5308}  &  \textcolor{red}{4664.73} \\ \hline  
\multicolumn{7}{c}{} \\ \hline
\multicolumn{1}{|c|}{Train} & \multicolumn{6}{c|}{238,148 obs.} \\
\hline
\multicolumn{1}{|c|}{Test} & \multicolumn{6}{c|}{59,537 obs.} \\ \hline
\end{tabular}
\caption{Model performances with column-wise median imputed data. All the algorithms are trained with five-fold cross validation. Only the \textit{BART-MIA} and the \textit{Logit CC} differ in the reported train and test sets since their cross-validation is respectively built  on the original dataset with missing values and on the complete-case version resulting from listwise deletion. All the metrics correspond to the five fold average. Time represents the average seconds required to train the model in each fold. Train and test represents the number of observations involved in each step of the cross-validation process.}
\end{table}

\begin{table}[H]
    \centering
    \begin{tabular}{|c|c|c|c|c|}
    \hline
\textit{Logit} & \textit{CTree} & \textit{RF} & \textit{XGBoost} & \textit{BART} \\ \hline
    0.0093    &    0.0303   &    0.1793    &    0.7031   &    0.0780 \\ \hline 
\end{tabular}
\caption{The SL distribution of the optimal coefficients for median imputation.}
\end{table}



\newpage
\subsection*{\textcolor{blue}{3) K-Nearest Neighbors (K-NN) median-based imputation}}
We perform imputation using the median of the $K = 5$ nearest neighbours of each case observation with missing values. We use the median for continuous variables and the mode for categorical ones. 

\begin{table}[H]
\centering
    \begin{tabular}{|l|c|c|c|c|c|r|}
\hline 
  &  ROC  &  PR  &  F1-Score  &  BACC  &  $R^2$  &  Time \\ \hline
\textcolor{blue}{\textit{Logit CC}} &  \textcolor{blue}{0.8798}  &  \textcolor{blue}{0.2047 } &  \textcolor{blue}{0.0788 } &  \textcolor{blue}{0.7477}  &  \textcolor{blue}{0.1065}  &  \textcolor{blue}{10.71} \\ \hline
\textit{Logit} &  0.8537  &  0.3101 &  0.1349  &  0.7158  &  0.1815 &  34.30  \\ \hline
\textit{Ctree}  &   0.9589  &  0.6758  &  0.1353  &  0.7719  &  0.4734  &  2115.82 \\ \hline
\textit{RF}   &  0.9856  &  0.8514  &  0.1914  &  0.8509  &  0.6496  &  810.73 \\ \hline
\textit{XGBoost} &   0.9650  &  0.6594  &  0.1737  &  0.8300  &  0.4492  &  2.49  \\ \hline
\textit{BART}  &  0.9733  &  0.7225  &  0.1267  &  0.7573  &  0.5152  &  5463.72  \\ \hline
\textit{SL} &   0.9894  &  0.8771  &  0.1271  &  0.7588  &  0.6988  &  13749.46  \\ \hline
\textcolor{red}{\textit{BART-MIA}} & \textcolor{red}{0.9768} &  \textcolor{red}{0.7468}  &  \textcolor{red}{0.1277}  &  \textcolor{red}{0.7599}  &  \textcolor{red}{0.5308}  &  \textcolor{red}{4664.73} \\ \hline  
\multicolumn{7}{c}{} \\ \hline
\multicolumn{1}{|c|}{Train} & \multicolumn{6}{c|}{238,148 obs.} \\
\hline
\multicolumn{1}{|c|}{Test} & \multicolumn{6}{c|}{59,537 obs.} \\ \hline
\end{tabular}
\caption{Model performances with K-NN imputed data. All the algorithms are trained with five-fold cross validation. Only the \textit{BART-MIA} and the \textit{Logit CC} differ in the reported train and test sets since their cross-validation is respectively built  on the original dataset with missing values and on the complete-case version resulting from listwise deletion. All the metrics correspond to the five fold average. Time represents the average seconds required to train the model in each fold. Train and test represents the number of observations involved in each step of the cross-validation process.}
\end{table}

\begin{table}[H]
    \centering
    \begin{tabular}{|c|c|c|c|c|}
    \hline
\textit{Logit} & \textit{CTree} & \textit{RF} & \textit{XGBoost} & \textit{BART} \\ \hline
 0  &  0  &  0.2653  &  0.7347  &  0  \\ \hline
\end{tabular}
\caption{The SL distribution of the optimal coefficients for uniform median imputation.}
\end{table}





\newpage
\subsection*{\textcolor{blue}{4) Uniform median sampling imputation}}
We impute the missing values of a variable $q$ by sampling from a continuous uniform distribution with bounded support on $[q_{.5}-s_n, \ q_{.5}+s_n]$, where $q_{.5}$ and $s_n$ are respectively the median and the sample standard deviation of the observed distribution of $q$.
\begin{table}[H]
\centering
    \begin{tabular}{|l|c|c|c|c|c|r|}
\hline 
  &  ROC  &  PR  &  F1-Score  &  BACC  &  $R^2$  &  Time \\ \hline
\textcolor{blue}{\textit{Logit CC}} &  \textcolor{blue}{0.8798}  &  \textcolor{blue}{0.2047 } &  \textcolor{blue}{0.0788 } &  \textcolor{blue}{0.7477}  &  \textcolor{blue}{0.1065}  &  \textcolor{blue}{10.71} \\ \hline
\textit{Logit} & 0.9061 & 0.2905 & 0.1261 & 0.7548 & 0.1573 & 27.63  \\ \hline
\textit{Ctree}  &  0.9187  &  0.3501  &  0.1618  &  0.8132  &  0.1985  &  1763.59     \\ \hline 
\textit{RF}   &   0.9698  &  0.6956  &  0.1396  &  0.7823  &  0.4609  &  753.82  \\ \hline
\textit{XGBoost} &  0.9617  &  0.6556  &  0.1671  &  0.8221  &  0.4390  &  2.77  \\ \hline
\textit{BART}  &   0.9678   &   0.6325   &   0.1268  &   0.7577   &   0.4236   &   4533.20 \\ \hline
\textit{SL} &    0.9767   &   0.7431   &   0.1269   &   0.7581   &   0.5280   &   15550.71   \\ \hline
\textcolor{red}{\textit{BART-MIA}} & \textcolor{red}{0.9768} &  \textcolor{red}{0.7468}  &  \textcolor{red}{0.1277}  &  \textcolor{red}{0.7599}  &  \textcolor{red}{0.5308}  &  \textcolor{red}{4664.73} \\ \hline  
\multicolumn{7}{c}{} \\ \hline
\multicolumn{1}{|c|}{Train} & \multicolumn{6}{c|}{238,148 obs.} \\
\hline
\multicolumn{1}{|c|}{Test} & \multicolumn{6}{c|}{59,537 obs.} \\ \hline
\end{tabular}
\caption{Model performances with uniform median imputed data. All the algorithms are trained with five-fold cross validation. Only the \textit{BART-MIA} and the \textit{Logit CC} differ in the reported train and test sets since their cross-validation is respectively built  on the original dataset with missing values and on the complete-case version resulting from listwise deletion. All the metrics correspond to the five fold average. Time represents the average seconds required to train the model in each fold. Train and test represents the number of observations involved in each step of the cross-validation process.}
\end{table}

\begin{table}[H]
    \centering
    \begin{tabular}{|c|c|c|c|c|}
    \hline
\textit{Logit} & \textit{CTree} & \textit{RF} & \textit{XGBoost} & \textit{BART} \\ \hline
  0  &  0.0720  &  0.2334  &  0.6936  &  0.0011  \\ \hline 
\end{tabular}
\caption{The SL distribution of the optimal coefficients for uniform median sampling imputation.}
\end{table}



\newpage

\begin{comment}
\subsection*{\textcolor{blue}{Unconditional mean imputation}}
\begin{table}[H]
\centering
\begin{tabular}{|l|c|c|c|c|c|r|}
\hline
   &  ROC   &   PR   &   F1-Score   &   BACC   &   $R^2$   &   Time \\ \hline 
\textit{BART}  &  0.9685  &  0.6672  &  0.1313  &  0.7665  &  0.4381  &  4361.47 \\ \hline \hline
\multicolumn{1}{|c|}{Train} & \multicolumn{6}{c|}{238,148 obs.} \\ \hline
\multicolumn{1}{|c|}{Test} & \multicolumn{6}{c|}{59,537 obs.} \\ \hline
\end{tabular}
\caption{BART performances (without MIA) with mean imputed data. The model is trained with five-fold cross validation. All the metrics correspond to the five fold average. Time time represents the average seconds required to train the model in each fold.}
\end{table}
\end{comment}



\newpage
\begin{figure}[H]
	\centering
	\caption{Transitions across deciles of risk: a visualization}
	\label{fig:sankey}
	\includegraphics[width=0.9\linewidth]{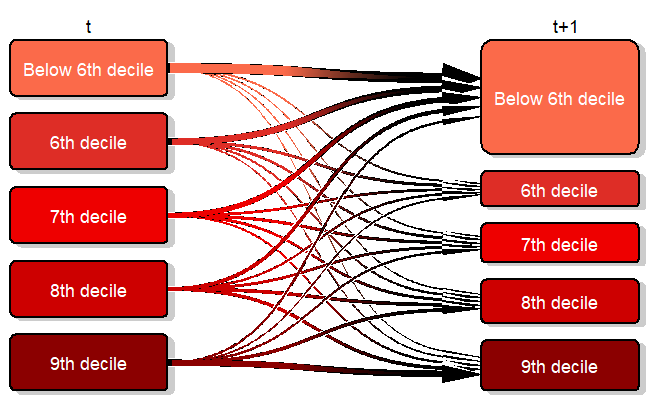}%
\end{figure}



\newpage
\section{Old analysis}
\subsection{Robustness and sensitivity checks}\label{sec:sensitivity}

The first robustness we implement is to check whether any imputation of missing values allows us to obtain better predictions after reverting to other techniques different from BART-MIA. We adopt a CART-based methodology \citep{buuren2010mice}, in the fashion of \citet{white2018imputation}, to fill in the missing financial accounts. We do not find any sensitive change in the ranking observed in Table \ref{tab:cc_analysis}. More in general, any finer tuning on the hyper-parameters does not seem to overturn the gap in performance between the BART-MIA and the other techniques.

A second check is done with respect to our choice of predictors. We want to be sure that nothing relevant is missing from our battery of predictors described in Table \ref{tab:table2}. Our sensitivity check is done in two steps by simulating synthetic predictors. In a first step, we generate a predictor whose correlation with the outcome of failure is as high as one of the best-observed predictors ($0.5$), but it is not significantly correlated with any of the other predictors  \cite[for more details on this methodology, see][]{bargagli2021assessing}. Hence, we check that its inclusion in a new augmented model affects unit-level predictions only in $0.88\%$ of cases (namely, just $0.88\%$ of the predictions of the augmented model are significantly different from the predictions of the original in (\ref{tree})). Then, we repeat the exercise by simulating a second synthetic predictor that is assumed correlated with both the outcome ($0.5$) and a predictor ($0.3$). In this case, unit-level predictions change only in 0.90\% of cases. We conclude that the original choice of predictors already captures the bulk of the signal in the data\footnote{Figure \ref{fig:sdm} provides a graphical intuition. It shows the standardized differences for the unit-level predictions of the augmented and the original model for 50 randomly selected observations. The standardized differences in the predictions do not deviate significantly, indicating no statistical difference between the predictions of the two models.}.

A third issue we want to address is the zero-inflated nature of our outcome variable. Any data set will structurally include a greater majority of incumbent firms that rarely exit from the market, i.e., the zeros. In contrast, the share of firms' failures is usually of a one-digit magnitude. For example, in the case of Italy, as from Table \ref{tab:italy_status}, only $5.7\%$ of firms failed in our period of analysis, in line with official figures from the Italian national statistics bureau. To clarify the nature of the problem, if we applied a methodology that predicted all the firms to fail in our data, we would still get an accuracy measure for correctly classified observations over total observations of 94.3\%. To deal with similar unbalanced outcomes, one could either under-sample the label that accounts for the largest majority of observations, or over-sample observations for the other label, as suggested in other applications \citep{gruszczynski2019,zhou2013performance}. In our case, we argue that any re-sampling method is sub-optimal because we know from Section \ref{sec:data}, Table \ref{tab:logit_missing}, and Appendix Table \ref{tab:chi-squared} that patterns of missing values are positively correlated with the outcome. For example, any under-sampling may induce a higher association between the missing observations and the failure of firms. In our framework, we argue that it is better to look at alternative goodness-of-fit measures that take into account unbalanced outcomes while keeping the sample intact.  See Table \ref{tab:cc_analysis} where we report PR, F1-score, and BACC, and we comment that BART-MIA predictions still show better accuracy.

\subsection{Old Missingness Plot}
\begin{figure}[H]
  \centering
  \caption{Patterns of missing values from a random subsample of 10,000 observations} %\footnotemark
  \label{fig:figure1}
\begin{subfigure}{\textwidth}
   \includegraphics[width=\linewidth]{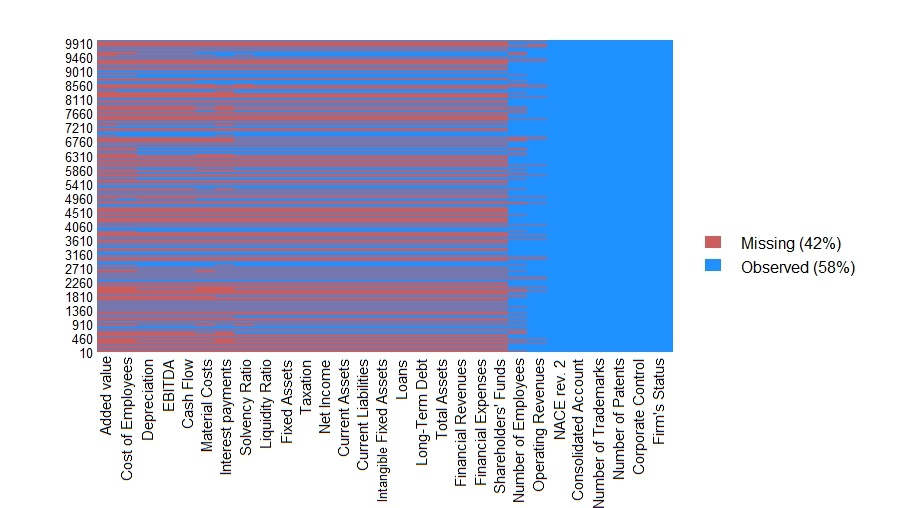}
   \caption*{Panel (A): Missing values of original financial accounts}
\end{subfigure}
\begin{subfigure}{\textwidth}
   \includegraphics[width=1\linewidth]{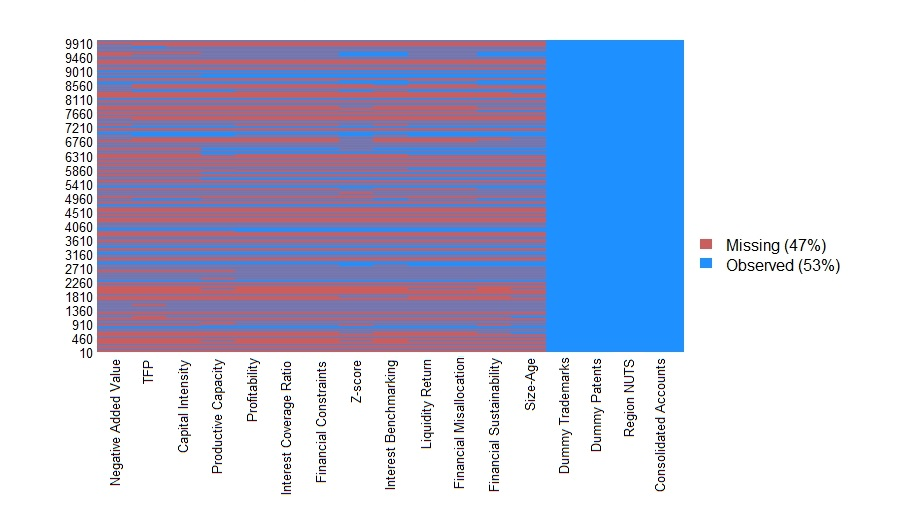}
   \caption*{Panel (B): Missing values of indicators based on original financial accounts.}
\end{subfigure}
\end{figure}

\begin{figure}[H]
	\centering
	\caption{Standardized Differences in the Predictions of Augmented and Original BART}
	\label{fig:sdm}
	\includegraphics[width=1\linewidth]{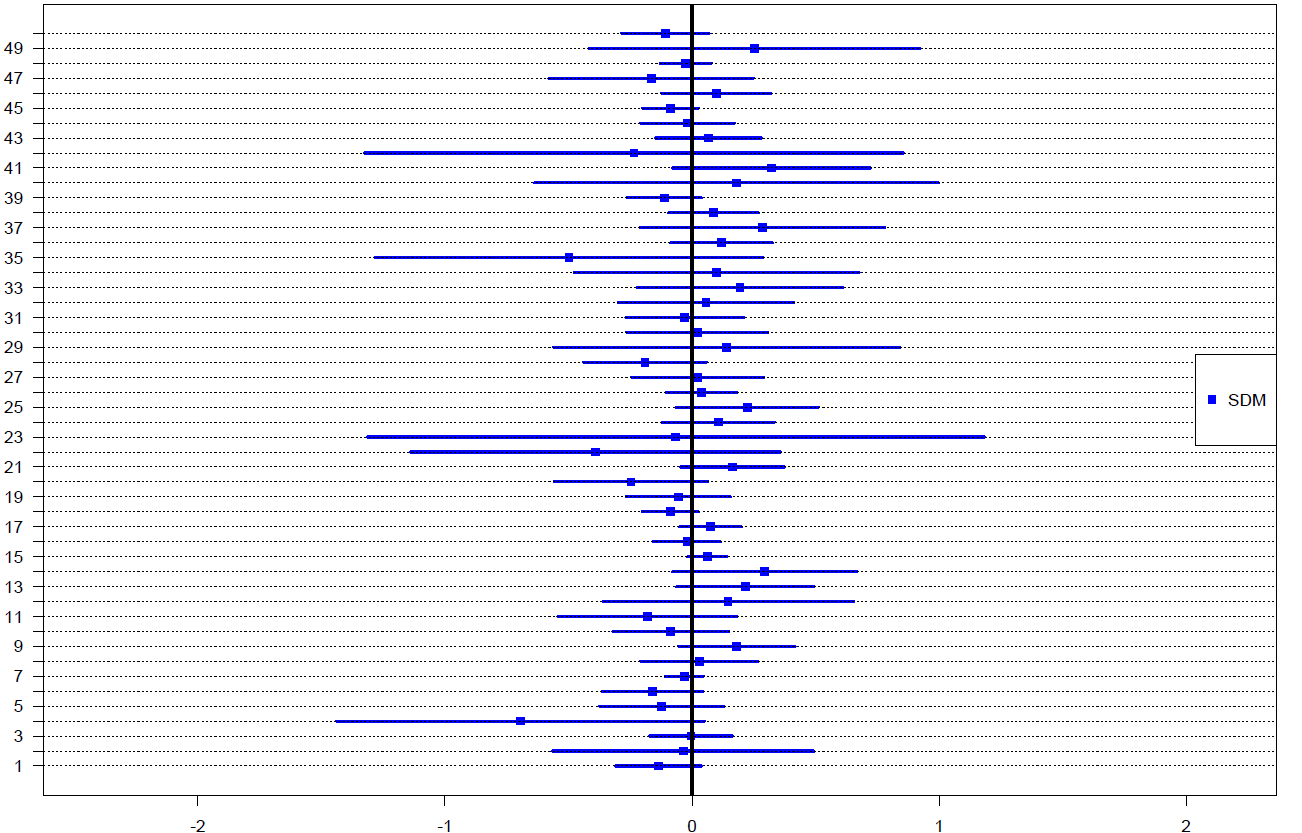}%
\end{figure}


\end{document}
